# Supplementary material for: A New Kind of Atlas of Zeolite Building Blocks
Source: arXiv:1907.03517 source file (2019-07-08)
Supplement: Supplementary file 1 [file SI.pdf]

# A New Kind of Atlas of Zeolite Building Blocks
# Supporting Information

Benjamin A. Helfrecht,[1] Rocio Semino,[2] Giovanni Pireddu,[3,1] Scott M. Auerbach,[4] and Michele Ceriotti[1]

[1]*Laboratory of Computational Science and Modeling, Institut des Matériaux, École Polytechnique Fédérale de Lausanne, 1015 Lausanne, Switzerland*

[2]*Institut Charles Gerhardt Montpellier UMR 5253 CNRS, Université de Montpellier, Place E. Bataillon, 34095 Montpellier Cedex 05, France*

[3]*Dipartimento di Chimica e Farmacia, Università degli Studi di Sassari, Via Vienna 2, 01700 Sassari, Italy*

[4]*Department of Chemistry and Department of Chemical Engineering, University of Massachusetts Amherst, Amherst, MA 01003 USA*

(Dated: July 7, 2019)

## I. SOAP PARAMETERS

Both the 3.5 Å and 6.0 Å SOAP descriptors employed 12 radial basis functions, a spherical harmonics band limit of 9, a cutoff transition width of 0.3, and an atomic Gaussian width of 0.3 (see the Quippy library reference for further information regarding the SOAP parameters, available at `https://libatoms.github.io/QUIP/descriptors.html`).

## II. COMPUTATIONAL TOOLS

The data analysis and and visualization for this study was performed in Python [1, 2] with the aid of the SciPy [3], NumPy [4, 5], scikit-learn [6], Atomic Simulation Environment (ASE) [7], quippy [8], and Matplotlib [9] packages in addition to Wolfram Mathematica 11.1 [10]. Atomic structure snapshots were created with Ovito [11] and Visual Molecular Dynamics (VMD) [12] with the Tachyon [13] rendering utility.

## III. SPARSE KERNEL METHODS

The sparse kernel methods that we use (KRR and KPCA) both approximate the full $N \times N$ kernel matrix $\mathbf{K}_{NN}$ with a reduced matrix $\mathbf{K}_{NM}$ that includes only a subset of the columns of $\mathbf{K}_{NN}$ in addition to $\mathbf{K}_{MM}$, the kernel matrix between only the $M$ "representative" feature vectors.

### A. Sparse Kernel Principal Component Analysis

One can approximate the full kernel $\mathbf{K}_{NN}$ using the eigendecomposition of its low rank approximation $\widetilde{\mathbf{K}}_{NN}$ [14] [15],

$$\mathbf{K}_{NN} \approx \widetilde{\mathbf{K}}_{NN} = \widetilde{\mathbf{U}}_{NN}\widetilde{\mathbf{\Lambda}}_{NN}\widetilde{\mathbf{U}}_{NN}^{T} \tag{1}$$

Under the Nyström approximation [14, 16], one can rewrite $\widetilde{\mathbf{K}}_{NN}$ as [14],

$$\widetilde{\mathbf{K}}_{NN} = \mathbf{K}_{NM}\mathbf{K}_{MM}^{-1}\mathbf{K}_{MN}. \tag{2}$$

Substituting $\mathbf{K}_{MM}$ for its eigendecomposition [17], one obtains,

$$\widetilde{\mathbf{K}}_{NN} = \mathbf{K}_{NM}\mathbf{U}_{MM}\mathbf{\Lambda}_{MM}^{-1}\mathbf{U}_{MM}^{T}\mathbf{K}_{MN}, \tag{3}$$

which can be rewritten as

$$\widetilde{\mathbf{K}}_{NN} = \mathbf{G}_{NM}\mathbf{G}_{MN}, \tag{4}$$

where $\mathbf{G}_{NM} = \mathbf{K}_{NM}\mathbf{U}_{MM}\mathbf{\Lambda}_{MM}^{-1/2}\mathbf{U}_{MM}^{T}$. Centering $\mathbf{G}_{NM}$ relative to its column means yields an approximation to the centered kernel matrix via Eqn. 4. Therefore, in the following, $\mathbf{G}_{NM}$ and $\widetilde{\mathbf{K}}_{NN}$ will be assumed to be centered. The eigendecomposition of $\mathbf{G}_{MN}\mathbf{G}_{NM} = \mathbf{V}_{MM}\mathbf{W}_{MM}\mathbf{V}_{MM}^{T}$ can then be used to approximate the $M$ largest eigenvectors of $\widetilde{\mathbf{K}}_{NN}$, i.e. [18, 19],

$$\widetilde{\mathbf{U}}_{NM} \approx \mathbf{G}_{NM}\mathbf{V}_{MM}\mathbf{W}_{MM}^{-1}. \tag{5}$$

Therefore, the KPCA projections can be computed as [20]

$$\widetilde{\mathbf{K}}_{NN}\widetilde{\mathbf{U}}_{NM} = \widetilde{\mathbf{K}}_{NN}\mathbf{G}_{NM}\mathbf{V}_{MM}\mathbf{W}_{MM}^{-1} \tag{6}$$

$$= \mathbf{G}_{NM}\mathbf{V}_{MM} \tag{7}$$

$$= \widetilde{\mathbf{U}}_{NM}\mathbf{W}_{MM} \tag{8}$$

### B. Sparse Kernel Ridge Regression

A sparse version of KRR can also be constructed from a subselected kernel matrix $\mathbf{K}_{NM}$. In this case, the solution to the KRR problem can be found by minimizing [21]

$$\frac{1}{2M}\|\mathbf{y}_N - \mathbf{K}_{NM}\mathbf{w}_M\|^2 + \lambda_1\mathbf{w}_M^T\mathbf{K}_{MM}\mathbf{w}_M, \tag{9}$$

with respect to the weights $\mathbf{w}_M$, for which the solution is [21]

$$\mathbf{w}_M = (M\lambda_1\mathbf{K}_{MM} + \mathbf{K}_{MN}\mathbf{K}_{NM})^{-1}\mathbf{K}_{MN}\mathbf{y}_N, \tag{10}$$

where $\mathbf{y}_N$ is a vector of the target properties. In our case, a structural kernel $\mathbf{K}_{LM}$ plays the role of the subselected kernel matrix, where each row $\mathbf{k}_M$ is the summation over a structure $S$ of the kernel between the environments comprising the structure and the $M$ representative

environments across the whole dataset [22],

$$\mathbf{k}_M = \sum_{\mathcal{A} \in S} \mathbf{k}_M^{\mathcal{A}}, \tag{11}$$

where $\mathcal{A} \in S$ denotes the atomic environments that belong to structure $S$. Furthermore, we apply a scaling $\delta = M \times \mathrm{Var}(\mathbf{y}_L) / \mathrm{Tr}(\mathbf{K}_{MM})$ to the target property vector $\mathbf{y}_L$ and to each kernel matrix, and we include an additional "jitter" parameter $\lambda_2 \mathbf{I}_{MM}$ so that the solution to our sparse KRR model is [22],

$$\mathbf{w}_M = (\lambda_1^2 \delta \mathbf{K}_{MM} + \lambda_2 \mathbf{I}_{MM} + \delta^2 \mathbf{K}_{ML} \mathbf{K}_{LM})^{-1} \delta^2 \mathbf{K}_{ML} \mathbf{y}_L, \tag{12}$$

where $\lambda_1$ and $\lambda_2$ are regularization parameters, and $\mathbf{y}_L$ is a vector containing the known structural properties for the $L$ structures. The parameter $\lambda_1$ was optimized along with the kernel width (in the case of Gaussian kernels) via five-fold cross validation; $\lambda_2$ was set to $10^{-16} \times \sigma$, where $\sigma$ is the largest eigenvalue of $\lambda_1^2 \delta \mathbf{K}_{MM} + \delta^2 \mathbf{K}_{ML} \mathbf{K}_{LM}$.

The optimal weights $\mathbf{w}_M$ can also be used to "decompose" the known structural property values $\mathbf{y}_L$ into contributions from the $N$ individual atomic environments $\hat{\mathbf{y}}_N$ across the whole dataset [22],

$$\hat{\mathbf{y}}_N = \mathbf{K}_{NM} \mathbf{w}_M. \tag{13}$$

## IV. RESULTS FOR THE 1,000-STRUCTURE SUBSET

Fig. S1 shows the learning curves for the classical and SOAP descriptors for the 1,000-structure subset, analogous to Fig. 3 in the main text. Fig. S2 gives a comparison of the SOAP-based and classical descriptors at comparable dimensionality for predicting the unit cell volume per atom and the energy per mol Si for the 1,000-structure subset. Fig. S2 is analogous to Fig. 4 in the main text. The learning curves of the 1,000-structure subset are similar to the results of the 10,000-structure subset for the first 1,000 training points.

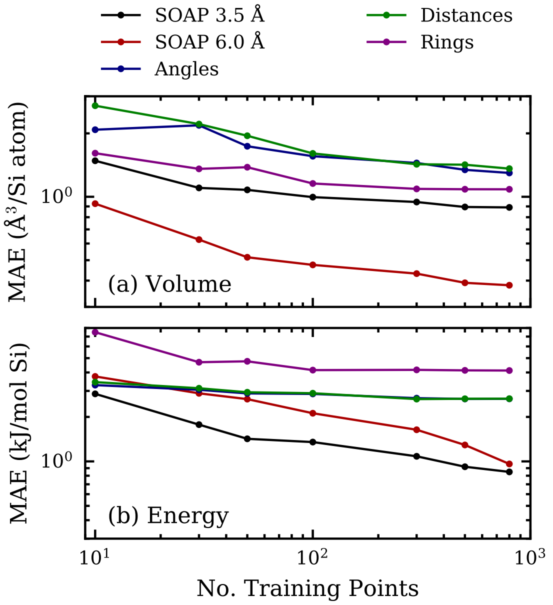


FIG. S1. Learning curves of the classical and SOAP descriptors for predictions of (a) volume per Si atom and (b) energy per mol Si for the 1,000-structure subset.

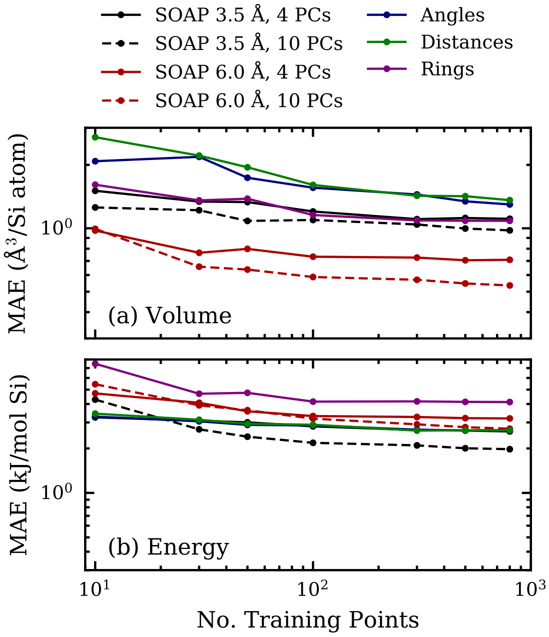


FIG. S2. Learning curves of classical and SOAP-KPCA descriptors with similar dimensionality for (a) predictions of volume per Si atom and (b) energy per mol Si for the 1,000-structure subset.

## V. SOAP KPCA

Figs. S3, S4, S5, and S6 show the learning curves for the prediction of zeolite volume per Si atom and energy per mol Si using the SOAP-KPCA representation with different numbers of principal components. As the number of principal components composing the representation is increased, the prediction becomes more accurate.

In the case of predicting the volume per atom, a SOAP-KPCA representation including 50 principal components performs similarly to a representation using all 500 of the FPS SOAP components (marked in the graph as "Original"). In the case of predicting the energy per mol Si, upwards of 100 principal components are required to match the prediction accuracy of the representation containing all 500 FPS SOAP vector elements.

The convergence of the prediction accuracy to that of the full FPS SOAP vector as more information (more principal components) are included into the KPCA representation also serves as a validation of the method: the KPCA-based representation can emulate the diversity of the SOAP vector and thus the local chemical environment.

A comparison can also be made between the prediction accuracy of the SOAP-KPCA representation and that of a classical descriptor with comparable information content (dimensionality). In this paradigm, a four-component SOAP-KPCA with 3.5 Å cutoff would contain roughly the same amount of information as the Si−O distance and Si−O−Si angle descriptors; a 10-component SOAP-KPCA with 6.0 Å cutoff would contain approximately the same amount of information as the ring-based descriptor, as ring sizes in our dataset range from 3–12.

When comparing the different representations in this manner, one finds that the performance of the distance- and angle-based descriptors is comparable to, or slightly worse than, the performance of a SOAP-KPCA descriptor including less than five principal components. The same is true for the ring-based descriptor in predicting the energy, but even a single-component 6.0 Å SOAP-KPCA descriptor outperforms the ring descriptor in predicting the volume per Si atom.

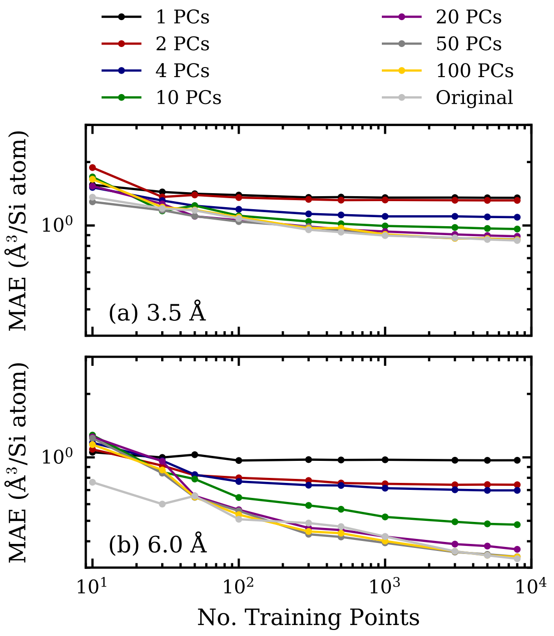


FIG. S3. Learning curves for the KPCA-SOAP descriptor for cutoff radii of 3.5 Å and 6.0 Å including different numbers of principal components for the 10,000-structure sample. Increasing the amount of information embedded into the descriptor (increasing the number of principal components) results in a better prediction of the average volume per Si atom

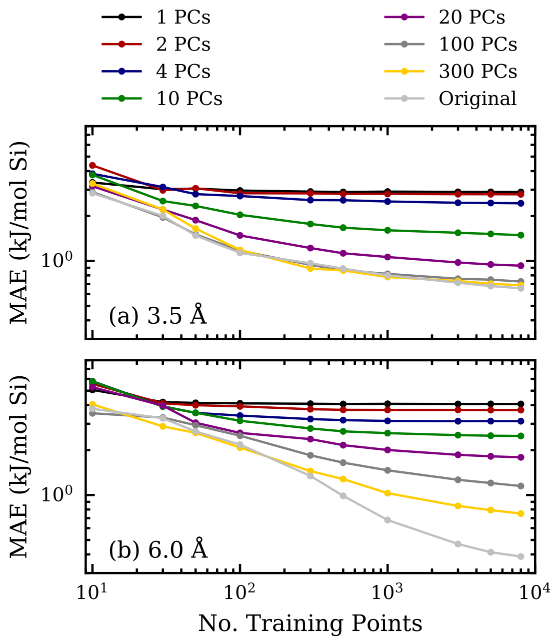


FIG. S4. Learning curves for the KPCA-SOAP descriptor for cutoff radii of 3.5 Å and 6.0 Å including different numbers of principal components for the 10,000-structure sample. Increasing the amount of information embedded into the descriptor (increasing the number of principal components) results in a better prediction of the average energy per mol Si

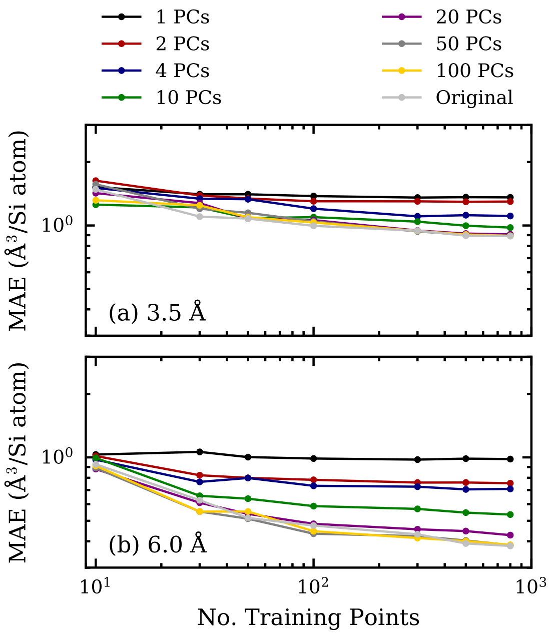


FIG. S5. Learning curves for the KPCA-SOAP descriptor for cutoff radii of 3.5 Å and 6.0 Å including different numbers of principal components for the 1,000-structure sample. Increasing the amount of information embedded into the descriptor (increasing the number of principal components) results in a better prediction of the average volume per Si atom

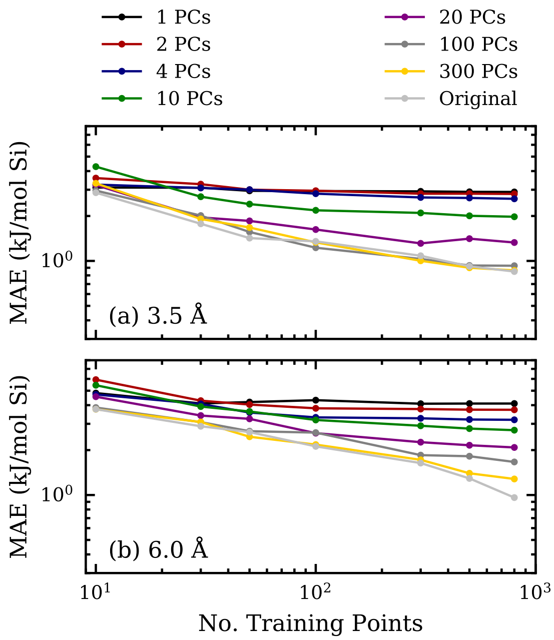


FIG. S6. Learning curves for the KPCA-SOAP descriptor for cutoff radii of 3.5 Å and 6.0 Å including different numbers of principal components for the 1,000-structure sample. Increasing the amount of information embedded into the descriptor (increasing the number of principal components) results in a better prediction of the average energy per mol Si

## VI. RING-BASED DESCRIPTORS

In terms of predicting the molar volume and energy, both King's definition and the shortest path definition perform very similarly. Figs. S7 and S8 show the learning curves for the ring descriptors built on the 1,000- and 10,000-structure samples. Two variations of the rings descriptor are examined. The "Distribution" ("Dist.") variant is the descriptor described in the main text: the $s$-th element of the feature vector for a given Si-centered environment is how many rings of size $s$ that include the central Si. The "Binary" ("Bin.") variant is a boolean version of the "Distribution" representation: the $s$-th element of the feature vector is 1 if the central Si participates in at least one ring of size $s$ and is 0 otherwise. As noted in the main article, the FPS of the ring descriptor often results in fewer than 2,000 unique environments. In these cases, only the unique feature vectors serve as representatives in the learning models. Consequently, the models based on the "binary" variants of the King and shortest path ring descriptors use 109 and 53 representatives (for the 1,000-structure sample) and 239 and 94 representatives (for the 10,000-structure sample), respectively; the model for the "distribution" variant of the shortest path ring counts in the 1,000-structure sample uses 763 representatives.

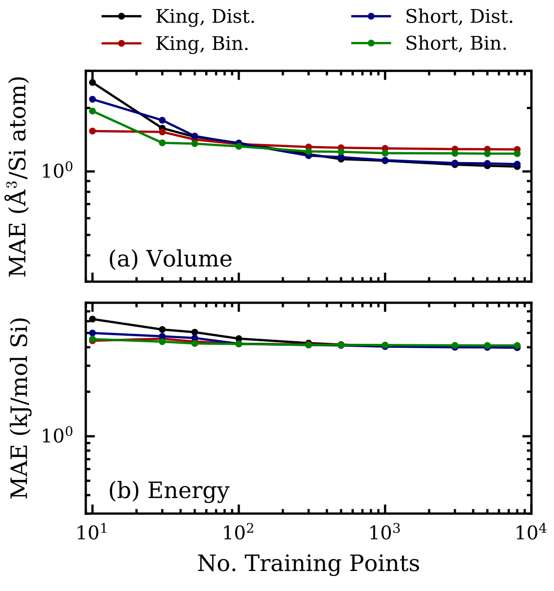


FIG. S7. Learning curves for the ring-based descriptors from the sample of 10,000 structures for predicting the volume per Si atom and the energy per mol Si.

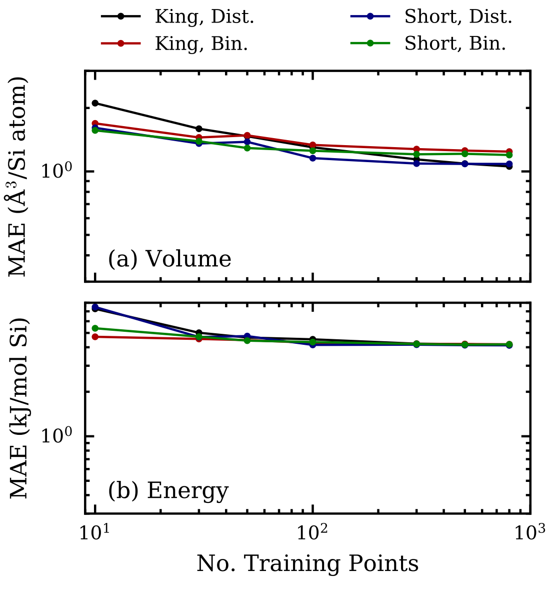


FIG. S8. Learning curves for the ring-based descriptors for the sample of 1,000 structures for predicting the volume per Si atom and the energy per mol Si.

## VII. PROPERTY CORRELATIONS

Figs. S9 is a plot of the Pearson correlation coeffients between the first 50 KPCs and the energy and volume as in Fig. 5 in the main text, but using a KPCA of SOAP representation with a 3.5 Å cutoff (instead of 6.0 Å). Similarly, Figs. S10 and S11 show the volume and energy correlations with the 3.5 Å and 6.0 Å SOAP-KPCA representations for the 1,000-structure subset.

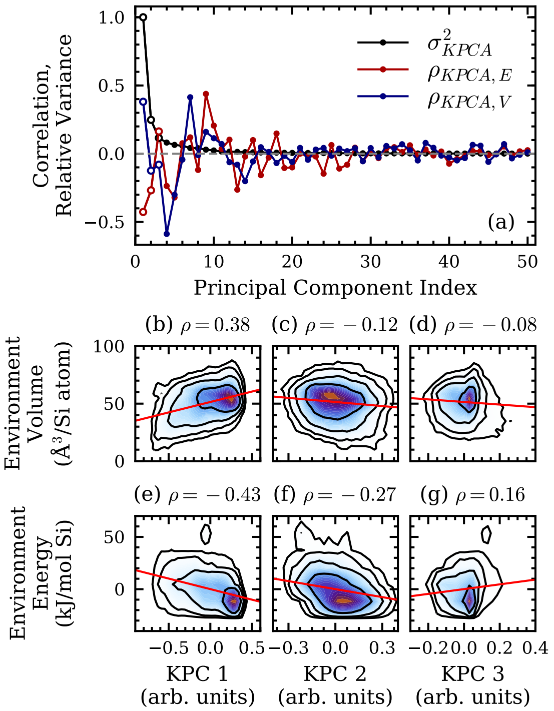


FIG. S9. (a) Pearson correlation coefficients between the first 50 KPCs of the 3.5 Å SOAP representation for the 10,000-structure sample and the decomposed environment volumes and energies. The relative variance in the KPCs at each of the first 50 components is also plotted. The correlation coefficients and relative variance of the first three components are highlighted with open symbols. (b)–(g) Kernel density estimation of all environments in KPC–property space with a least squares fit to the data to show the correlations in more detail. The value of the Pearson correlation coefficient is given above each contour set.

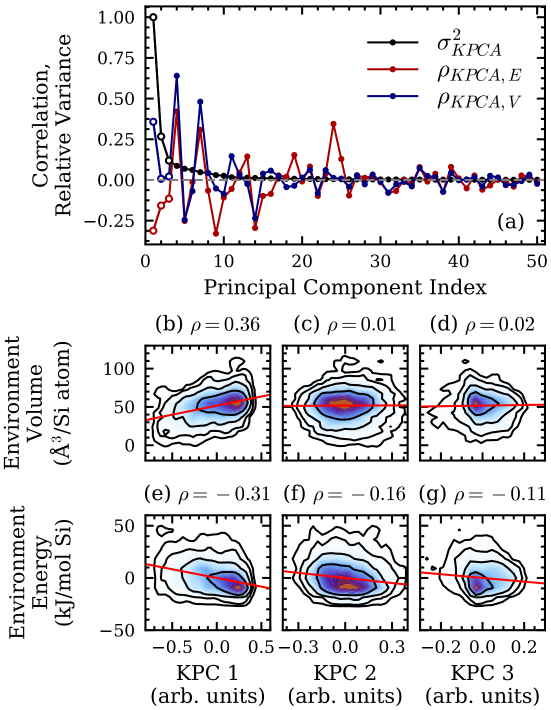


FIG. S10. (a) Pearson correlation coefficients between the first 50 KPCs of the 3.5 Å SOAP representation for the 1,000-structure sample and the decomposed environment volumes and energies. The relative variance in the KPCs at each of the first 50 components is also plotted. The correlation coefficients and relative variance of the first three components are highlighted with open symbols. (b)–(g) Kernel density estimation of all environments in KPC–property space with a least squares fit to the data to show the correlations in more detail. The value of the Pearson correlation coefficient is given above each contour set.

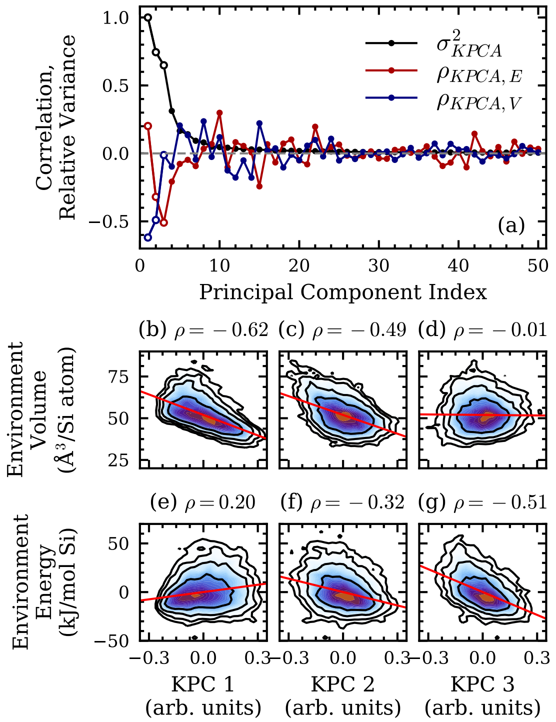


FIG. S11. (a) Pearson correlation coefficients between the first 50 KPCs of the 6.0 Å SOAP representation for the 1,000-structure sample and the decomposed environment volumes and energies. The relative variance in the KPCs at each of the first 50 components is also plotted. The correlation coefficients and relative variance of the first three components are highlighted with open symbols. (b)–(g) Kernel density estimation of all environments in KPC–property space with a least squares fit to the data to show the correlations in more detail. The value of the Pearson correlation coefficient is given above each contour set.

[1] T. E. Oliphant, Computing in Science and Engineering **9**, 10 (2007).

[2] K. J. Millman and M. Aivazis, Computing in Science and Engineering **13**, 9 (2011).

[3] E. Jones, T. Oliphant, P. Peterson, *et al.*, "SciPy: Open source scientific tools for Python," (2001–).

[4] T. E. Oliphant, *A Guide to NumPy* (Trelgol Publishing, USA, 2006).

[5] S. van der Walt, S. C. Colbert, and G. Varoquaux, Computing in Science and Engineering **13**, 22 (2011).

[6] F. Pedregosa, G. Varoquaux, A. Gramfort, V. Michel, B. Thirion, O. Grisel, M. Blondel, P. Prettenhofer, R. Weiss, V. Dubourg, J. Vanderplas, A. Passos, D. Cournapeau, M. Brucher, M. Perrot, and Édouard Duchesnay, Journal of Machine Learning Research **12**, 2825 (2011).

[7] A. H. Larsen, J. J. Mortensen, J. Blomqvist, I. E. Castelli, R. Christensen, M. Duak, J. Friis, M. N. Groves, B. Hammer, C. Hargus, E. D. Hermes, P. C. Jennings, P. B. Jensen, J. Kermode, J. R. Kitchin, E. L. Kolsbjerg, J. Kubal, K. Kaasbjerg, S. Lysgaard, J. B. Maronsson, T. Maxson, T. Olsen, L. Pastewka, A. Peterson, C. Rostgaard, J. Schitz, O. Schtt, M. Strange, K. S. Thygesen, T. Vegge, L. Vilhelmsen, M. Walter, Z. Zeng, and K. W. Jacobsen, Journal of Physics: Condensed Matter **29**, 273002 (2017).

[8] N. Bernstein, G. Csányi, J. Kermode, A. Bartók-Pártay, L. Bartók-Pártay, F. Bianchini, A. Butenuth, M. Caccin, S. Cereda, A. Comisso, T. Daff, S. T. John, C. Gattinoni, G. Moras, L. Mones, A. Nichol, D. Packwood, L. Pastewka, G. Peralta, I. Solt, O. Strickson, W. Szlachta, C. Varnai, and S. Winfield, "libatoms/quip," https://github.com/libAtoms/QUIP.

[9] J. D. Hunter, Computing in Science and Engineering **9**, 90 (2007).

[10] W. R. Inc., "Mathematica, Version 11.1," Champaign, IL, 2017.

[11] A. Stukowski, Modelling and Simulation in Materials Science and Engineering **18**, 015012 (2009).

[12] W. Humphrey, A. Dalke, and K. Schulten, Journal of Molecular Graphics **14**, 33 (1996).

[13] J. Stone, *An Efficient Library for Parallel Ray Tracing and Animation*, Master's thesis, Computer Science Department, University of Missouri-Rolla (1998).

[14] C. K. I. Williams and M. Seeger, in *Advances in Neural Information and Processing Systems 13*, edited by T. K. Leen, T. G. Dietterich, and V. Tresp (MIT Press, 2001) pp. 682–688.

[15] The SAS/IML 15.1 User's Guide [23] also provides a comprehensive overview of the same sparse KPCA algorithm outlined here.

[16] C. T. H. Baker, *The Numerical Treatment of Integral Equations* (Clarendon Press, 1977).

[17] M. Li, W. Bi, J. T. Kwok, and B.-L. Lu, IEEE Transactions on Neural Networks and Learning Systems **26**, 152 (2015).

[18] K. Zhang, I. W. Tsang, and J. T. Kwok, in *Proceedings of the 25th International Conference on Machine Learning*, ICML '08 (ACM, New York, NY, USA, 2008).

[19] C. Fowlkes, S. Belongie, F. Chung, and J. Malik, IEEE Transactions on Pattern Analysis and Machine Intelligence **26**, 214 (2004).

[20] M. E. Tipping, in *Advances in Neural Information and Processing Systems 13*, edited by T. K. Leen, T. G. Dietterich, and V. Tresp (MIT Press, 2001) pp. 633–639.

[21] A. J. Smola and B. Schökopf, in *Proceedings of the Seventeenth International Conference on Machine Learning*, ICML '00 (Morgan Kaufmann Publishers Inc., San Francisco, CA, USA, 2000) pp. 911–918.

[22] M. Ceriotti, M. J. Willatt, and G. Csányi, in *Handbook of Materials Modeling*, edited by W. Andreoni and S. Yip (Springer, Cham, 2018).

[23] SAS Institute Inc., *SAS/IML ®15.1 User's Guide* (SAS Institute Inc., Cary, NC, 2018).
